# Supplementary material for: Reinforcement-learning-based actuator selection method for active flow control
Source: arXiv:2209.14895 source file (2022-09-29)
Supplement: Supplementary file 1 [file Z0_TDbased_Vi.tex]

\subsection*{Bellman-backup-based value function estimation}\label{app:TD_estimation}

The Bellman backup equation is the backbone of reinforcement learning. It formulates the following self-consistency condition for the value function:
\begin{align*}
    V^\pi(s_t) = r_t + \gamma*(1-d_t)*V^\pi(s_{t+1})
\end{align*}

Let $\pi^i$ be the current policy where the $i^{th}$ action component is clipped
