# Supplementary material for: Reinforcement-learning-based actuator selection method for active flow control
Source: arXiv:2209.14895 source file (2022-09-29)
Supplement: Supplementary file 2 [file Z1_AS_algo_pseudoCode.tex]

\section{Action-sparisty seeking algorithm pseudo-code}
$\theta$ are parameters for $\pi$ and $\phi$ for $V$
\input{algo/action_sparse_vi_algo}
